# Supplementary material for: Linear Distances between Markov Chains
Source: arXiv:1605.00186 source file (2016-06-23)
Supplement: Supplementary file 1 [file appendix.tex]

\section{Additional Definitions from Section~\ref{sec:pos}}

For arbitrarily large $k$, the analysis will depend on whether the chains $\Mc_1$ and $\Mc_2$ are \emph{pathological} or not, in the following sense. Intuitively, a pathological chain can be thought of as the chain which contains a BSCC bisimilar to a deterministic cycle.

\begin{definition}\rm
A chain is \emph{pathological}, if it accepts some infinite word with positive probability, i.e., $\exists \sigma\in {\Sigma}^w. \Pm(\sigma)>0$. 
\end{definition}

\begin{lemma}\rm
If $\Mc$ contains an $\infty$-deterministic state, it is pathological.
\label{lem:pat}
\end{lemma}

\begin{proof}\rm
Let $s\in S$ be an $\infty$-deterministic state and let $\pi=s_0,s_1,\dots,s_n,s$ be one of the shortest paths from the initial state in $\Mc$ ($s_0$) to $s$ with positive probability. 
Let $w\in \Sigma^\omega$ be the infinite word such that $\Pr(w\mid s)=1$. 
Let $w':=L(\pi).w$ (concatenation of word $L(\pi)$ and $w$). Then $\Pr(w')\geq \Pr(\pi)>0$.
\end{proof}

\begin{definition}\rm
A BSCC is \emph{pathological}, if all its states are $\infty$-deterministic. 
%\przemek{IMHO: is pathological if all its states  are $k$-deterministic, for every $k\geq 1$}\jan{both is correct, $\infty$ looks simpler to me. What is "initial"? We could say "if there is a $\infty$-deterministic state (and then all are)"}
\end{definition}

Notice that a pathological BSCC is bisimilar to a (deterministic) cycle.
The following lemma is useful for supporting the intuition on the relation between a pathological chain and a pathological BSCC, even though we do not use it directly in the subsequence proofs.

\begin{lemma} \rm
A chain is {pathological} if and only if it contains a pathological BSCC. %\tanja{this we don't need in the current proofs}
\end{lemma}

\begin{proof}\rm 
One direction follows from Lemma~\ref{lem:pat} - if there is a pathological BSCC, there is by definition an $\infty$-deterministic state and the chain is pathological. 
Assume that $\Mc$ is pathological and it does not contain a BSCC with all states $\infty$-deterministic, that is, each BSCC has at least one finitely branching state. 
But then, by Kolmogorov zero-one law, % \tanja{add reference of refine?}, 
all infinite words visit a branching state infinitely often, and consequently they all have measure $0$. 
\end{proof}

\begin{theorem}\rm 
If $\Mc$ is a non-pathological chain of size $n$ and $N=n^2-1$, then for every $\epsilon>0$ and $K>N\frac{\ln(\epsilon)}{\ln(1-\pmin^{N})}$, 
for any word $\sigma\in \Sigma^\omega$, the probability of its $K$-prefix is bounded by $\epsilon$, that is,
$\Pm(\sigma|_K)<\epsilon$.
\label{thm:sd}
\end{theorem}

\begin{proof}\rm
First notice that, if each state in a chain is $2$-branching (has at least two successors with different labels),
for any infinite trace $\sigma\in \Sigma^\omega$, the probability of its $(k+1)$-prefix $\sigma|_{k+1}$ is smaller than the probability of its $k$-prefix $\sigma|_k$, at least by factor $(1-\pmin)$, 
that is 
$$
\hbox{(if all states $2$-branching)\;\;\;}\forall \sigma\in Ap^\omega,\forall k\geq 1.\Pm(\sigma|_{k+1})\leq\Pm(\sigma|_k)(1-\pmin).
$$%\przemek{I would remove the part for n=2 and keep the general case}
Let now $N=n^2-1$, where $n$ is the size of $\Mc$. % the bigger of the chains $\Mc_1$ and $\Mc_2$.
% length of the longest label-deterministic sequence in the chains $\Mc_1$ and $\Mc_2$. 
%By the assumption that both chains are not pathological, $n$ must be finite (an infinite label-deterministic sequence in either of the chains implies the existence of a pathological BSCC) and smaller than the size of the chain.
%
Then, by Lemma~\ref{lem:br}, each state is $N$-branching and, by Lemma~\ref{lem:bound}, any word of length $N$, starting in any state $s\in S$ has probability at most $1-\pmin^{n^2-1}=1-\pmin^N$.
As a consequence, the probability of a word obtained by extending any word with $N$ labels decreases at least with a factor $(1-\pmin^N)$. 
Then, the argument above extends to
$$
\hbox{(since all states $(N+1)$-branching)\;\;\;}\forall \sigma\in \Sigma^\omega,\forall k\geq 1.\Pm(\sigma|_{k+N})\leq\Pm(\sigma|_{k})(1-\pmin^N),
$$
%Let $\sigma|_{k}= \overline{a_1\ldots a_{k}}$ and $\sigma|_{k+n}= \overline{a_1\ldots a_{k}u_1\ldots u_n}$. 
%
%Since chains are not pathological, there must be at least one sequence of states
%$w=s_1\ldots s_{n(k+1)}$, such that 
%$L(s_1\ldots s_{n(k+1)}) = \sigma|_{n(k+1)}$ and
%$\Pm(s_1\ldots s_{n(k+1)}) \leq \Pm(s_1\ldots s_{nk})\pmin^{n-1}(1-\pmin)$ (label-branching happens at least once in every $n$ steps). 
which follows from 
\begin{align*}
\Pm(\sigma|_{k+N})
& = \sum_{L(s_1\ldots s_{k}s_1'\ldots s_{N}')=\sigma|_{k+N}} \Pm(s_1\ldots s_{k}s_1'\ldots s_{N}')\\
& = \sum_{L(s_1\ldots s_{k})=\sigma|_{k}} \Pm(s_1\ldots s_{k})\left(\sum_{s_1'\ldots s_{N}'\in \sigma|_{k+1,\ldots, N}}\Pm(s_1'\ldots s_{N}'\mid s_k)\right)\\
& \leq (1-\pmin^{N})\sum_{L(s_1\ldots s_{k})=\sigma|_{k}}  \Pm(s_1\ldots s_{k}), \hbox{ by Lemma~\ref{lem:br} and \ref{lem:bound}}\\
& = (1-\pmin^{N})\Pm(\sigma|_k).
\end{align*}
For an example, see Figure~\ref{fig:ex_with_thm2}. %\przemek{Some explanation?}
Finally, for $K>N\frac{\ln(\epsilon)}{\ln(1-\pmin^{N})}$ 
by repeatedly applying the argument above, we obtain that
$
%\dist_{K}(\Mc_1,\Mc_2)\leq \max_{\sigma\in \Sigma^{K}} \{\Pm_1(w),\Pm_2(w)\}
\Pm(\sigma|_{K})\leq (1-\pmin^{N})^{K}=\epsilon$.

\end{proof}

\begin{corollary} \rm (to Theorem~\ref{thm:sd}) 
Let $\Mc_1$ and $\Mc_2$ be two finite, non-pathological Markov chains, $n$ is the size of larger of the chains and $N=n^2-1$. 
Then, for every $\epsilon>0$ and $K>N\frac{\ln(\epsilon)}{\ln(1-\pmin^{N})}$, $\dist_{K}(\Mc_1,\Mc_2)<\epsilon$. 
In other words, for traces longer than $N\frac{\ln(\epsilon)}{\ln(1-\pmin^{N})}$, the distance is bounded by $\epsilon$.
Moreover, computing $\dists(\Mc_1,\Mc_2)$ with $\epsilon$-precision can be done by computing the distance for all lengths up to $K$: 
\begin{align}
|\dists(\Mc_1,\Mc_2)-\max_{k\leq K}\dist_k (\Mc_1,\Mc_2)|\leq \epsilon.
\label{eq:gen}
\end{align}
In particular, if the distance is achieved for some $k<K$, it is then computed precisely.
%\przemek{I would move the last sentence out of the theorem statement; also $K>n\frac{\ln(\epsilon)}{\ln(1-\pmin^{n})}$}
%
%Concretely, if $n$ is the size of larger of the chains, it suffices to take
%$K:=\frac{\ln(\epsilon)}{\ln(1-\pmin^{n-1})}$.
%\log_{(1-p)}\epsilon$.
\end{corollary}

\section{Safety and liveness}
The definitions below are based on ``Principles of Model Checking'' and an unpublished book by Tom on model checking.

Let $\Ap$ be a set of atomic propositions. A \emph{linear-time property} $P$ (or $\omega$-language) is $P \subseteq \Ap^\omega$.
The set of all (finite) prefixes of the words in $P$ is denoted by $pref(P)$:
\[ pref(P) = \{\hat{\sigma} \in \Ap^* ~|~ \hat{\sigma} \text{ is a finite prefix of a word in } P \}. \]
The closure of an LT property $P$ is the set of infinite words, such that all their prefixes are in $pref(P)$:
\[ closure(P) = \{\sigma \in \Ap^\omega  ~|~ pref(\sigma) \subseteq pref(P)\}.\]

In general, safe properties have only finite counterexamples, while live properties have only infinite counterexamples.

\begin{definition}[Safe property]
	A LT property $P$ is safe if $P = closure(P)$. 
\end{definition}

\begin{definition}[Alternative def.~of safety]
	A LT property $P$ is safe if for all words $\sigma \in \Ap^\omega \setminus P$ there exists a  ``bad'' prefix $\hat{\sigma}$ of $\sigma$ that cannot be extended to any word in $P$:
	\[P \cap \{ \sigma' \in \Ap^\omega ~|~ \hat{\sigma} \text{ is a prefix of } \sigma' \} = \emptyset. \]
\end{definition}

\begin{definition}[Live property]
	A LT property $P$ is live if $pref(P) = \Ap^*.$
\end{definition}

\begin{definition}[Safety -- livness decomposition]
	Every LT property $P$ can be written as $P = P_s \cap P_l$, where
	$P_s$ is a safe and $P_l$ is live.
	
	\begin{proof}
		Let $P_s = closure(P)$ and $P_l = P \cup (\Ap^\omega \setminus P_s)$.
	\end{proof}
\end{definition}

\section{$\omega$-Regular languages}

\begin{definition}
	A language is $\omega$-regular if it is accepted by some non-deterministic B\"{u}chi automata.
\end{definition}

A $\omega$-regular $\lang$ language can be expressed as 
\[ \lang = L_1\cdot L_2^\omega \cup \cdots \cup L_{n-1}\cdot L_n^\omega,  \]
where $L_1, \cdots, L_n$ are regular languages and $L^\omega$ is an infinite concatenation of words from $L$.

\newpage

\section{FW}

\subsection{Kullback-Leibler divergence}

If $P$ and $M$ are discrete probability measures on a common measurable space $(\Omega,{\cal F})$, then
\[
D(P||M) = \sum_{\omega\in\Omega} p(\omega) \ln \frac{p(\omega)}{m(\omega)}.
\]

In particular, if $P_{0:k}$ and $M_{0:k}$ are $k$-prefix trace distributions for two different chains defined with matrices $P$ and $M$ over the same state space and for $s\in S$, denote by 
$\pi_s(t)$ (resp. $\pi'_s(t)$) the probability of being in state $s$ at time $t$ in the first (resp. second) chain, then
\[
D(P_{0:k}||M_{0:k}) =  D(\pi(0)||\pi'(0))+\sum_{i=0}^{k-1} \sum_{s\in S} \pi_s(t)\sigma(s),
\]
where 
\[
\sigma(s):= \sum_{s'\in S} P_{s,s'}\ln\frac{P_{s,s'}}{M_{s,s'}},
\]
hence the KL divergence for prefix trace distributions can be computed from the transient distribution and the transition matrices. 
KL divergence is always non-negative, 
but it is not a metric: it is non-symmetric, and it does not satisfy the triangle inequality.
It is still often used as a measure of similarity between probability distributions. 
A common technical interpretation is that KL divergence is the coding penalty associated with selecting the candidate distribution to approximate the correct distribution \cite{Cover}. 

In case there is a unique stationary distribution for both chains, then the \emph{divergence rate} is the average divergence over infinite traces: 
\[
\tilde{D}(P||M) =  \lim_{n\rightarrow \infty}\frac{1}{n}D(P_{0:n}||M_{0:n}) , 
\]

As a side note: the KL divergence of measure ${\mathsf P}$ with respect to measure ${\mathsf M}$ (discrete- or continuous-) is defined as the supremum of relative entropy with respect to all possible discrete measurements (partitions): 
$D(P||M) = \sup_{f} H_{{\mathsf P}||{\mathsf M}}(f)$,
where the \emph{relative entropy} of $f$ with measure ${\mathsf P}_{f}$, with respect to the measure ${\mathsf M}$ is
$H_{{\mathsf P}||{\mathsf M}}(f) =
\sum_{a\in{\cal R}(f)} p_{f}(a) \ln \frac{p_{f}(a)}{m_{f}(a)}$ if ${\mathsf P}_{f}$ is absolutely continuous with respect to ${\mathsf M}_{f}$ and otherwise $H_{{\mathsf P}||{\mathsf M}}(f) =\infty$ (${\cal R}(f)$ being the range of measurement $f$).

\subsection{Wasserstein-Kantorovich distance} % \jan{please fill in the def.+Maas's work}}

If $\mu$ and $\nu$ are probability measures on a common measurable space,
%$(\Omega,{\cal F})$,
then the Wasserstein distance is defined as 
\[
W_p(\mu, \nu) = \left(\inf_{(X,Y)\in\Gamma_{\mu,\nu}} E[d(X,Y)^p]\right)^{1/p},
\]
where $E[Z]$ denotes the expected value of a random variable $Z$ and $\Gamma(\mu,\nu)$ are all joint distributions of the random variables $X$ and $Y$ with marginals $\mu$ and $\nu$ respectively.

For Markov chains $\Mc_1$ and $\Mc_2$, if $\llbracket\Mc\rrbracket_t$ denotes the probability measure in semantics with time horizon $t$, the Wasserstein distance is
\[ \distw(\Mc_1, \Mc_2,t) = W_p(\llbracket\Mc_1\rrbracket_t,\llbracket\Mc_2\rrbracket_t).\]

For $p=1$, Wasserstein distance is a special case of `earth-mover's distance', denoting the minimum cost of turning one pile of dirt to another, where the cost is the amount of dirt moved times the distance by which it is moved. 

Metrics on the domain space:
\begin{itemize}
	\item $2^{-n}$ where $n$ is the length of the common prefix; standard; reflects changes at the beginning
	\item apply $=$ point-wise, compute mean-payoff; reflects long-run behaviour
	\item as above but discounted payoff; you have a knob to shift your preference between earlier and later parts
	\item metric of Jan Maas?
\end{itemize}

\section{Further ideas}

Apart from the already mentioned deterministic B\"uchi with all states final (closed sets) and all NBA/DRA ($\omega$-regular sets), further automata-based classes include DRA of \emph{size at most $k$} for a fixed $k\in\Nset$, or NBA with \emph{all accepting states sinks}, corresponding to reachability in a finite automaton and to regular unions of cones $\{L\Sigma^\Omega\mid L\text{ is regular}\}$, being between clopen and open sets.\jan{This should be a lot simpler than infinite words since there is no recurrent behaviour.}

Interesting fragments:
\jan{notes:}
\begin{itemize}
	\item $\X,\wedge$ - like supremum difference distance, seems approximable (trick with branching and no-branching)
	\item $\X,\wedge,\vee$ - inapproximable due to explicit representation of the distinguishing event in the inapproximabililty proof for total variation
	\item LTL($\F,\G$) -- maybe can simulate $\X$ in some cases, seems inapproximable?
	\item LTL($\F\G,\G\F$) -- simple analysis of BSCCs
\end{itemize}

\subsection{Problem space}

The problem defined in section \ref{def:pd} has more dimensions:
\begin{enumerate}
	\item Which distance we consider?
	\item Do we assume some granularity of the Markov chains? \jan{``finite precision''}
	\item Whether we compare two black-box models, or rather a black-box with a white-box. \jan{do we know of any difference?}
	\item Do we observe only labels or also states? \jan{states}
	\item Can we enforce the initial state or just start the system from its initial distribution? \jan{the latter; the former leads to branching distances}
\end{enumerate}

% Let 
% We consider the following problem: given two  Markov chains $\Mc_1, \Mc_2$, threshold value $\epsilon\geq 0$, and indifference region $\delta\geq 0$, and bounds $\alpha, \beta\in [0;1]$, we want to decide between two hypothesis $H_0$ and $H_1$, where
% \[ H_0: \dist(\Mc_1, \Mc_2) \leq \epsilon - \delta \qquad H_1: \dist(\Mc_1, \Mc_2) > \epsilon + \delta\]
% s.t.\ the Type-I and Type-II errors are bounded by $\alpha, \beta$, respectively.
% %Alternatively, we consider a variation of the problem, where $\Mc_1$ is white-box.

\tanja{For later -- phrase the general problem -- we aim for an SMC algorithm for testing the hypothesis that some distance is in a given interval
	\[H_0: \;\;\dist(\Mc_1,\Mc_2) \in I \;\;\; \text{or just lower/upper bound}
	\]
	by only running the chains (both black box).
	So the answer should be such that the hypothesis is accepted with given upper bound on the Type I error (if it holds with probability at least $1-\alpha$).
}

%From now on, we assume that $\epsilon - \delta > 0$, otherwise the problem cannot be solved for any measure when at least one MC is a black-box.
------

Trace distance - for non-equivalent chains compute ditances for length 1, 2,...
When a non-zero one is reached, say $\epsilon$, it induces $k$ such that nothing longer than $k$ has to be checked. 
If all further up to $k$ are smaller then output $\epsilon$, otherwise the bigger number.

\subsection{Automata}

Working hypothesis: we can learn both MC, and bound the difference in probability that any automata of size $k$ can create. Decomposition of automata into livness and safety part could help. 

\begin{itemize}
	\item acyclic DFA: can check the $k$-prefix
	\item with self-loops: can check presence of (not necessarily connected) $k$-subwords and alphabet in each segment
	\item cyclic: ...???
	\jan{I'll try to refine, DFA are easier than our previous attempts at B\"uchi}
\end{itemize}

Another simple option could be all-states-accepting DBAs.

\end{document}
